# Supplementary material for: AssetHarvester: A Static Analysis Tool for Detecting Secret-Asset Pairs in Software Artifacts
Source: arXiv:2403.19072 source file (2024-11-20)
Supplement: Supplementary file 1 [file Appendix.tex]

\input{Tables/QuestionCountPerYear}
\input{Tables/tagskeywords}
\input{Tables/FinalAnswerMappingsTables}
